# Supplementary material for: GraphIt: A High-Performance DSL for Graph Analytics
Source: arXiv:1805.00923 source file (2018-10-22)
Supplement: Supplementary file 1 [file appendices.tex]

\myparagraph{Fusing iterative graph kernels} Program
structure optimizations enable optimization across iterative graph kernels, such as
PageRank and Eigenvector Centrality as shown below.
\punt{(Listing~\ref{lst:kernel_fusion})}

\begin{lstlisting}[ label={lst:kernel_fusion}, language=graphit,escapechar=|]
...
func updateEdge(src : Vertex, dst : Vertex)
    NewRank[dst] += OldRank[src] / OutDegree[src];
end
func updateEdgeEigenVector(src : Vertex, dst : Vertex)
    NewEc[dst] += OldEc[src];
end
func main()
    #l1# for i in 1:10
        #s1# edges.apply(updateEdge);
        vertices.apply(updatePRVertex);
    end
    #l2# for i in 1:10
         #s1# edges.apply(updateEdgeEigenVector);
         vertices.apply(updateECVertex);
    end
end
schedule:
program->fuseFields({``OldRank'', ``OutDegree'', ``OldEc''})
->fuseForLoop(``l1'', ``l2'', ``l3'')
->fuseApplyFunctions(``l3:l1:s1'', ``l3:l2:s1'', ``fusedFunc'')
->configApplyParallelization(``l3:l1:s1'', ``vertex-parallel'')
->configApplyDirection(``l3:l1:s1'', ``DensePull'');
    
\end{lstlisting}

The goal is to fuse together the iterative kernels into a single
iterative kernel by fusing together the loops, functions, and 
vectors that are always accessed together (OldRank, OutDegree, and
OldEc) to significantly boost spatial locality.  
We use the command \fuseForLoop, which fuses
together two for-loops, identified by the labels \textbf{l1} and
\textbf{l2}, and replaces them with a new for-loop \textbf{l3}.  If
the index ranges of the original for-loops are not the same, two
additional for-loops, \textbf{l1\_prologue} and \textbf{l1\_epilogue},
will be generated to ensure the correctness of the program.  The fused
loop replace the original \textbf{l1} loop.  
The command \fuseApplyFunctions{} creates a
new edgeset \apply{} to replace the \textbf{l3:l1:s1} 
statement.  In Section~\ref{sec:eval}, we show that fusion of multiple
iterative kernels with similar access patterns can boost the
performance of the application by up to 60$\%$.
